# Supplementary material for: Beyond Flat Text: Dual Self-inherited Guidance for Visual Text Generation
Source: arXiv:2501.05892 source file (2025-03-22)
Supplement: Supplementary file 1 [file X_suppl.tex]

\clearpage
\setcounter{page}{1}
\maketitlesupplementary

\section{Additional Background}
\label{sup:bac}

\paragraph{Latent Diffusion Models.}
The Latent Diffusion Models (LDM) denoise a noisy vector $z_t$ to $z_0$ that is mapped to an image $x_0$ through an autoencoder, based on a text prompt $y$. To sequentially remove the noise $\varepsilon$, a network $\varepsilon_{\theta}$ is trained to minimize the loss: 
\begin{equation}
\label{eq:Diffusion}
\mathcal{L} = \mathbb{E}_{z_0,y,\varepsilon\sim\mathcal{N}(0,1),t} || \varepsilon - \varepsilon_\theta(z_t, t, c(y)) ||_2^2 ,
\end{equation}
where the $c(y)$ is the conditioning embedding of the prompt $y$, $z_t$ is a noisy vector obtained by adding noise to $z_0$ according to the timestep $t$. During inference, provided a random noise vector $z_T$, the trained network iteratively removes the predicted noise to produce a latent $z_0$ for $T$ steps. Namely, we employ popular DDIM sampling \cite{song2020denoising} for inference: 
\begin{equation}
\label{eq:DDIM}
\begin{aligned}
    z_{t-1} = &\sqrt{\alpha_{t-1}}\underbrace{(\frac{z_t-\sqrt{1-\alpha_t\epsilon_{\theta}(z_t)}}{\sqrt{\alpha_t}})}_{\text{predicted $z_0$}} \\ 
    &+ \sqrt{1-\alpha_{t-1}-\sigma^2_{t} \cdot \epsilon_{\theta}(z_t)}.
\end{aligned}
\end{equation}
The DDIM Sampling in general combines the predicted $z_0$ and $z_t$ to obtain the $z_{t-1}$. We mainly analyze the predicted $x_0$ that is decoded 
from predicted $z_0$ in the rest of the section.

\paragraph{Adaptive Instance Normalization.} The Adaptive Instance Normalization (AdaIN) \cite{huang2017arbitrary} is previously adopted in the task of style transfer. It substitutes mean and standard deviation of the activations from each CNN \cite{krizhevsky2012imagenet} filter of the original image with those of the style image as follows:
\begin{equation}
\label{eq:AdaIN}
\begin{aligned}
    {\rm AdaIN}(x, y) = \sigma(y)(\frac{x-\mu(x)}{\sigma(x)})+\mu(y),
\end{aligned}
\end{equation}
% where $x$ and $y$ stands for the activation of a CNN filter from the content image and style image, $\mu(\cdot)$ and $\sigma(\cdot)$ are channel-wise mean and standard deviation. Even though in \cite{huang2017arbitrary}, it is necessary to train a decoder for the style-transferred image. 
where $x$ and $y$ stand for the activation of a CNN filter from the content image and style image, $\mu(\cdot)$ and $\sigma(\cdot)$ are channel-wise mean and standard deviation. Masui \etal \cite{masui2024harnessing} further prove that the AdaIN can be directly applied to the LDM without any additional training for style transfer.

\section{Analysis of Predicted $x_0$}

As shown in \cref{fig:inter}, AnyText can produce clear and intact visual texts in structure even in the first inference step. However, the prediction becomes blurry and wrong once tilted as in the second column. The following columns show the effectiveness of our method. SRB can improve the structure. The SIB further improves the structure but produces visual texts that are not coherent with the background. More visualization of intermediates of SRB and SIB are shown in \cref{fig:SRB_inter}. 

\section{Full Algorithm}

The complete algorithm is represented as \cref{alg:ours}. 

\begin{table*}[t]
\centering
\begin{tabular}{cccccccccccc}
\toprule
    \multirow{2}*{Language}                 & \multirow{2}*{$\lambda$} & \multirow{2}*{$\rho$} & \multicolumn{4}{c}{Sen.ACC}   & \multicolumn{4}{c}{NED}       & \multirow{2}*{CLIP score} \\ 
    \cmidrule(l){4-7} \cmidrule(l){8-11}
        ~                 &                        &                     & easy  & medium & hard & total & easy  & medium & hard & total &            \\
    \midrule             
\multirow{7}{*}{English} & -0.5                   & \cellcolor{gray!30}{0.5}                 & 71.33 & 35.51 & 6.14  & 44.88 & 87.23 & 62.98 & 22.79 & 64.11 & 0.3005     \\
                        & 0.5                    & \cellcolor{gray!30}{0.5}                 & \underline{71.25} & 37.25 & 6.60  & \textbf{45.43} & \textbf{87.54} & 64.42 & 24.56 & 65.10 & \underline{0.3027}     \\
                        & \cellcolor{gray!30}{0.5}                    & 0.25                & \textbf{71.37} & 37.11 & 5.32  & \underline{45.12} & 87.10 & 63.80 & 21.19 & 63.85 & \textbf{0.3036}     \\
                         & \cellcolor{gray!30}{0.5}                    & 0.75                & 69.60 & \underline{38.39} & \textbf{7.16} & 45.10 & \underline{87.33} & \textbf{65.54} & \textbf{25.94} & \textbf{65.65} & 0.3006     \\
                         & \cellcolor{gray!30}{0.5}                    & 1.25                & 61.48 & 35.16 & 6.33  & 40.18 & 85.38 & 63.73 & \underline{25.44} & 64.11 & 0.3008     \\
                         & \cellcolor{gray!30}{0.5}                    & 1.5                 & 69.47 & \textbf{38.92} & 6.48  & 45.01 & 87.23 & 65.03 & 25.43 & \underline{65.34} & 0.3009     \\
                         & \cellcolor{gray!30}{0.5}                    & 1.75                & 69.19 & 38.17 & 6.56  & 44.70 & 87.18 & \underline{65.31} & 25.40 & 65.39 & 0.3011     \\
                         & \cellcolor{gray!30}{0.5}                    & 2.0                 & 68.88 & 37.96 & \underline{6.71}  & 44.53 & 87.07 & 64.85 & 25.26 & 65.17 & 0.3009     \\
                         \midrule
\multirow{7}{*}{Chinese} & -0.5                   & \cellcolor{gray!30}{0.5}                 & 68.61 & 35.02 & 7.54  & 49.28 & 95.17 & 85.23 & 66.05 & 87.29 & 0.3067     \\
                         & 0.5                    & \cellcolor{gray!30}{0.5}                 & \underline{69.22} & 35.58 & 8.55 & \underline{49.96} & \underline{95.37} & \underline{85.85} & 68.77 & \textbf{88.08} & \underline{0.3071}     \\
                         & \cellcolor{gray!30}{0.5}                    & 0.25                & \textbf{71.35} & 35.42 & 6.16  & \textbf{50.70} & \textbf{95.46} & \textbf{85.88} & 67.37 & 87.86 & \textbf{0.3076}     \\
                         & \cellcolor{gray!30}{0.5}                    & 0.75                & 66.12 & \underline{37.79} & \underline{10.66} & 49.05 & 94.54 & 85.77 & \underline{70.38} & 87.89 & 0.3058     \\
                         & \cellcolor{gray!30}{0.5}                    & 1.25                & 64.28 & \textbf{38.11} & \textbf{10.57} & 48.03 & 94.31 & 86.14 & \textbf{71.58} & \underline{88.07} & 0.3060     \\
                         & \cellcolor{gray!30}{0.5}                    & 1.5                 & 63.85 & 37.05 & 9.83  & 47.40 & 94.24 & 85.52 & 70.26 & 87.64 & 0.3061     \\
                         & \cellcolor{gray!30}{0.5}                    & 1.75                & 65.53 & \textbf{38.11} &  10.29 &  48.12 & 94.29 & \underline{85.85} & 70.21 & 87.73 & 0.3064        \\
                         & \cellcolor{gray!30}{0.5}                    & 2.0                 & 65.02 & 35.91 & 10.11 & 47.88 & 94.44 & 85.37 & 69.78 & 87.63 & 0.3059     \\  
\hline 
\end{tabular}
\caption{\textbf{Detailed sensitivity analysis for $[\lambda, \rho]$.}}
% \vspace{-10pt}
\label{tab:supp_sensi}
\end{table*}

\begin{algorithm}[t]
\SetAlgoLined
\textbf{Input:} A text prompt $y$, an input position image $l_p$, a flat reference position image $\Tilde{l}_p$ and a set of iterations for refinement $\left\{t_1, \ldots , t_k\right\}$ and a trained Visual Text Generation Model $\mathcal{M}$ .\\ %intermediate results of DDIM inversion $z^*_T,\ldots,z^*_0$ (using $w=1$).\\
\textbf{Output:} Denoised vector $z_0$ .\\
 %Let $(s_{Normal},s_T,s_{T-1},\ldots,s_1)$ be a sequence of random seeds\; 
\vspace{1mm} \hrule \vspace{1mm}
Render the glyph image $l_g$ and compute its latent $z_g$; \\
Compute the reference latent $z^{f}_0$; \\
Rotate and crop $z^{f}_0$ to get $z_f$ according to the transformation from $\Tilde{l}_p$ to $l_p$; \\
\For{$t=T,T-1,\ldots,1$}{
   \If{$t \in \left\{t_1, \ldots , t_k\right\}$}{
   $\Tilde{z}_t \gets {\rm AdaIN} (z_f,z_t) \odot l_p+z_t\odot(1-l_p)$; \\
   $\hat{z}_t \gets \rho {\rm AdaIN}(z_g,z_t) + (1 - \rho) \Tilde{z}_t$;\\
   % $z_t \gets \lambda (\rho {\rm AdaIN} (z_{f},\hat{z}_t) +(1-\rho) \hat{z}_t) \odot l_p + z_t$; \\
   $\ddot{z}_t \gets (\kappa_t\lambda \hat{z}_t + (1-\kappa_t) z_t) \odot l_p + z_t \odot (1-l_p)$; \\
   Set $z_t \gets \ddot{z}_t$; \\
   }
   Set $z_{t-1} \gets \mathcal{M}(z_t,y,t,l_p,l_g)$; \\
}

\textbf{Return} $z_0$ 

\caption{STGen}
\label{alg:ours}
\end{algorithm}

\section{Additional Results}

Here we provide additional results of our method. Our code will be released upon acceptance.

\begin{table*}[t]
\centering
\begin{tabular}{cccccccccc}
\toprule
    \multirow{2}*{Method}  & \multicolumn{4}{c}{Sen.ACC}   & \multicolumn{4}{c}{NED}       & \multirow{2}*{CLIP score} \\ 
    \cmidrule(l){2-5} \cmidrule(l){6-9}
    ~      & easy  & medium & hard & total & easy  & medium & hard & total &            \\
    \midrule
    AnyText & 66.00 & 26.38 & 2.02 & 44.78 & 94.48 & 81.37 & 59.38 & 84.74 & 0.3064 \\
    AnyText+Art-Finetuned & \underline{68.73} & \underline{28.99} & \underline{3.31} & \underline{47.20} & \underline{94.78} & \underline{83.30} & \underline{60.01} & \underline{85.46} & \textbf{0.3073} \\
    AnyText+Ours &  \textbf{69.22} & \textbf{35.58} & \textbf{8.55} & \textbf{49.96} & \textbf{95.37} & \textbf{85.85} & \textbf{68.77} & \textbf{88.08} & \underline{0.3071} \\
    \hline 
\end{tabular}
\caption{\textbf{Results of Art Finetuned AnyText in Chinese set.}}
\label{tab:supp_art_finetuned}
\end{table*}

\subsection{Additional Quantitative Results}\label{sec:more_results}

\paragraph{Hyper-parameters Sensitivity.} As shown in the \cref{tab:supp_sensi}, our method shows robustness in hyper-parameters change. The best performance is obtained when $\rho$ is 0.75 at the hard level. But the method achieves the best performance in the easy level of Chinese and English set when $\rho$ is 0.25. To ensure fairness, we choose the performance when $\rho$ is 0.5 which has a balanced performance for comparison. 

\paragraph{Comparison with finetuned model.} We increase the weight of ArT~\cite{chng2019icdar2019} Dataset in the AnyWord-3M Dataset \cite{tuo2023anytext} to train the model. ArT contains texts in arbitrary shapes in the image. We use the same set of training parameters in the AnyText \cite{tuo2023anytext} training phrase. % It takes 2 NVIDIA A40 GPUs and trained for about 30 minutes. 
The results are shown in the \cref{tab:supp_art_finetuned}, although in the Chinese evaluation set, we obtain a better performance compared to the original AnyText,% we observe a severe performance drop in English evaluation set. Comparing to the finetuned results, 
our method still produces the best results. 

\paragraph{Efficiency analysis.} When generating a batch of four images with 20 inference steps, AnyText requires 13.183 seconds, whereas our method takes 28.338 seconds. Both approaches are configured consistently, as described in \cref{sec:imple}.

% \TODO{Add an experiment of changing $\kappa_t$. But is it necessary? Discuss this with Zixun later.}

% \begin{table}[t]
% \footnotesize
%     \centering
%     \begin{tabular}{lccccccc}
%     \toprule
%        \multirow{2}*{Method}  & \multicolumn{3}{c}{English} & \multicolumn{3}{c}{Chinese} \\
%        \cmidrule(l){2-4} \cmidrule(l){5-7}
%        ~ & SEN.ACC & NED & FID & SEN.ACC & NED & FID \\
%        \midrule
%        AnyText & 72.39 & 87.67 & \textbf{33.54} & 69.23 & 83.96 &  \textbf{31.58} \\
%        w/ Ours & \textbf{75.53} & \textbf{89.38} & 37.46 & \textbf{70.00} & \textbf{84.57} &  35.06 \\
%        \bottomrule
%     \end{tabular}
%     \vspace{-5pt}
%     \caption{\textbf{Evalutaion on vanilla AnyText Benchmark.}}
%     \vspace{-5pt}
%     \label{tab:anytextbench}
% \end{table}

% \paragraph{Results on vanilla AnyText Benchmark.} As shown in \cref{tab:anytextbench}, our method is comparable to the original AnyText on AnyText Benchmark. Our method does not affect AnyText original performance. 

\subsection{Additional Qualitative Results}

\paragraph{Choice of $\lambda$}
We can observe in \cref{fig:lam} that when $\lambda$ is in the range of $(0,0.5]$ we can achieve background with more diversity and in the range of $[-0.5,0)$ the diversity of texts is increased consistent with what we mentioned in \cref{sec:imple}. 

% \paragraph{Coherence with Background.} As shown in \cref{fig:back}, thanks to the rich semantic information contained in the latent with flat visual texts, we can generate visual texts that are perfectly blended in with the background. The text `Harvest' in the bottom right is more harmonious with the background and is closest to the description ``interwoven".

\paragraph{Visual Text Diversity.} As shown in the first row of \cref{fig:diversity}, with proper control, our method can generate texts in various styles and colors. The second row shows that the generated visual texts remain accurate under 2 different image styles. The third row demonstrates the robustness of our method under different challenging masks. The fourth row shows our ability to generate various visual texts using the same prompt.  

\paragraph{Additional Comparison with baseline.} % \todo{The full qualitative results are shown in the \cref{fig:full_qualitative}}. 
We provide further qualitative comparisons in three groups: simple slanted cases (\cref{fig:add0}), simple curved cases (\cref{fig:add1}), and complex scenarios (\cref{fig:add2}). Our method consistently produces high-quality images featuring accurate visual text.

\section{Benchmark Details.} 
\label{sup:detailofbenchmark}

As shown in \cref{fig:benchmark_detail}, the benchmark we created inherited the prompt and the lines of text as much as possible. Besides, our benchmark evaluates the generation ability of the model for generating visual texts in various angles, sizes, and languages.

\section{Details of User Study}
\label{sup:detailofuser}

An illustration of our user study is provided in \cref{fig:user_study}. Since the captions in the English (LAION) set are often hard for users to understand (\eg ``carousel of carousel of carousel of carousel of carousel of carousel of carousel of carousel of carousel of carousel of carousel"). To produce meaningful prompts that can help the user understand, we employ LLMs to generate image prompts for user study. Here we provide a simplified template of our instructions and examples:
\begin{tcolorbox} 
{\slshape 
\textcolor{NavyBlue}{\textbf{1.Task instruction}}\\
I am working on a text-to-image generation task, where I need to generate images from given Text Prompts. Each Prompt should include a scene description and contain one or two sets of words that need to be present in the image, enclosed in double quotes. \\
\textcolor{Plum}{\textbf{2. Examples}}

\begin{itemize}
    \item A raccoon stands in front of the blackboard with the words ``Deep Learning" written on it
    \item A crayon drawing by the child, a snowman with a Santa hat, pine trees, outdoors in heavy snowfall, titled ``Snowman".
    \item ......
\end{itemize}
%\begin{center}
%    ......
%\end{center}% \centerline{......} \\
\textcolor{ForestGreen}{\textbf{3.Trigger CoT reasoning ability of LLMs}} \\
Reasoning: This task is very important to me. 
Let's think step by step......
}
\end{tcolorbox}

\section{Limitations}

Our method still inherits the problems of the baseline AnyText, such as the unsatisfactory ability to generate texts on a small scale or to generate texts in a specific font. Restricted by the latent size, our method may not acquire accurate texts when the text region is too small.

\begin{figure*}[t]
    \centering
    \includegraphics[width=1.0\linewidth]{images/interv3.pdf}
    \vspace{-10pt}
    \caption{\textbf{Comparison of predicted $x_0$ under different inference steps in various masks.} \textit{The first column is the AnyText intermediate results under a flat mask, AnyText can predict the structure of the texts at the very early stage of inference. The rest of the columns show intermediates in a slanted mask using AnyText and other operations using different methods. %SRB stands for Structure-rectifying Branch and SIB stands for Structure-refining Branch. 
    Our method can revise the originally wrong texts and harmonize the background. }}%\YX{To be honest, this figure is not good, lacking of beautify. Could we replace it}}
    \vspace{-10pt}
    \label{fig:inter}
\end{figure*}

\begin{figure*}[t]
    \centering
    \includegraphics[width=1.0\linewidth]{images/SRB_inter.pdf}
    \vspace{-10pt}
    \caption{\textbf{Demonstration of SRB and SIB intermediate results.} \textit{}}
    \vspace{-10pt}
    \label{fig:SRB_inter}
\end{figure*}

\begin{figure*}[t]
    \centering
    \includegraphics[width=1.0\linewidth]{images/lambda.pdf}
    \vspace{-10pt}
    \caption{\textbf{Results under different lambda.} \textit{When $\lambda$ is -0.5, we obtain colorful and styled visual texts in the first column. When $\lambda$ is 0.5, we produce images with rich background. When $\lambda$ is 0, the method degrades to vanilla AnyText. }}
    \vspace{-10pt}
    \label{fig:lam}
\end{figure*}

\begin{figure*}
    \centering
    \includegraphics[width=1.0\linewidth]{images/diversityv3.pdf}
    \caption{\textbf{Diversity demonstration.}\textit{The first row demonstrates various fonts and colors a single prompt can generate. The second row shows that the same texts with different prompts can still generate coherent and reasonable images. We use different masks in the third row. The fourth row illustrates the ability to simply change the language of the generated texts.}}
    \label{fig:diversity}
\end{figure*}

\begin{figure*}
     \centering
     \includegraphics[width=1.0\linewidth]{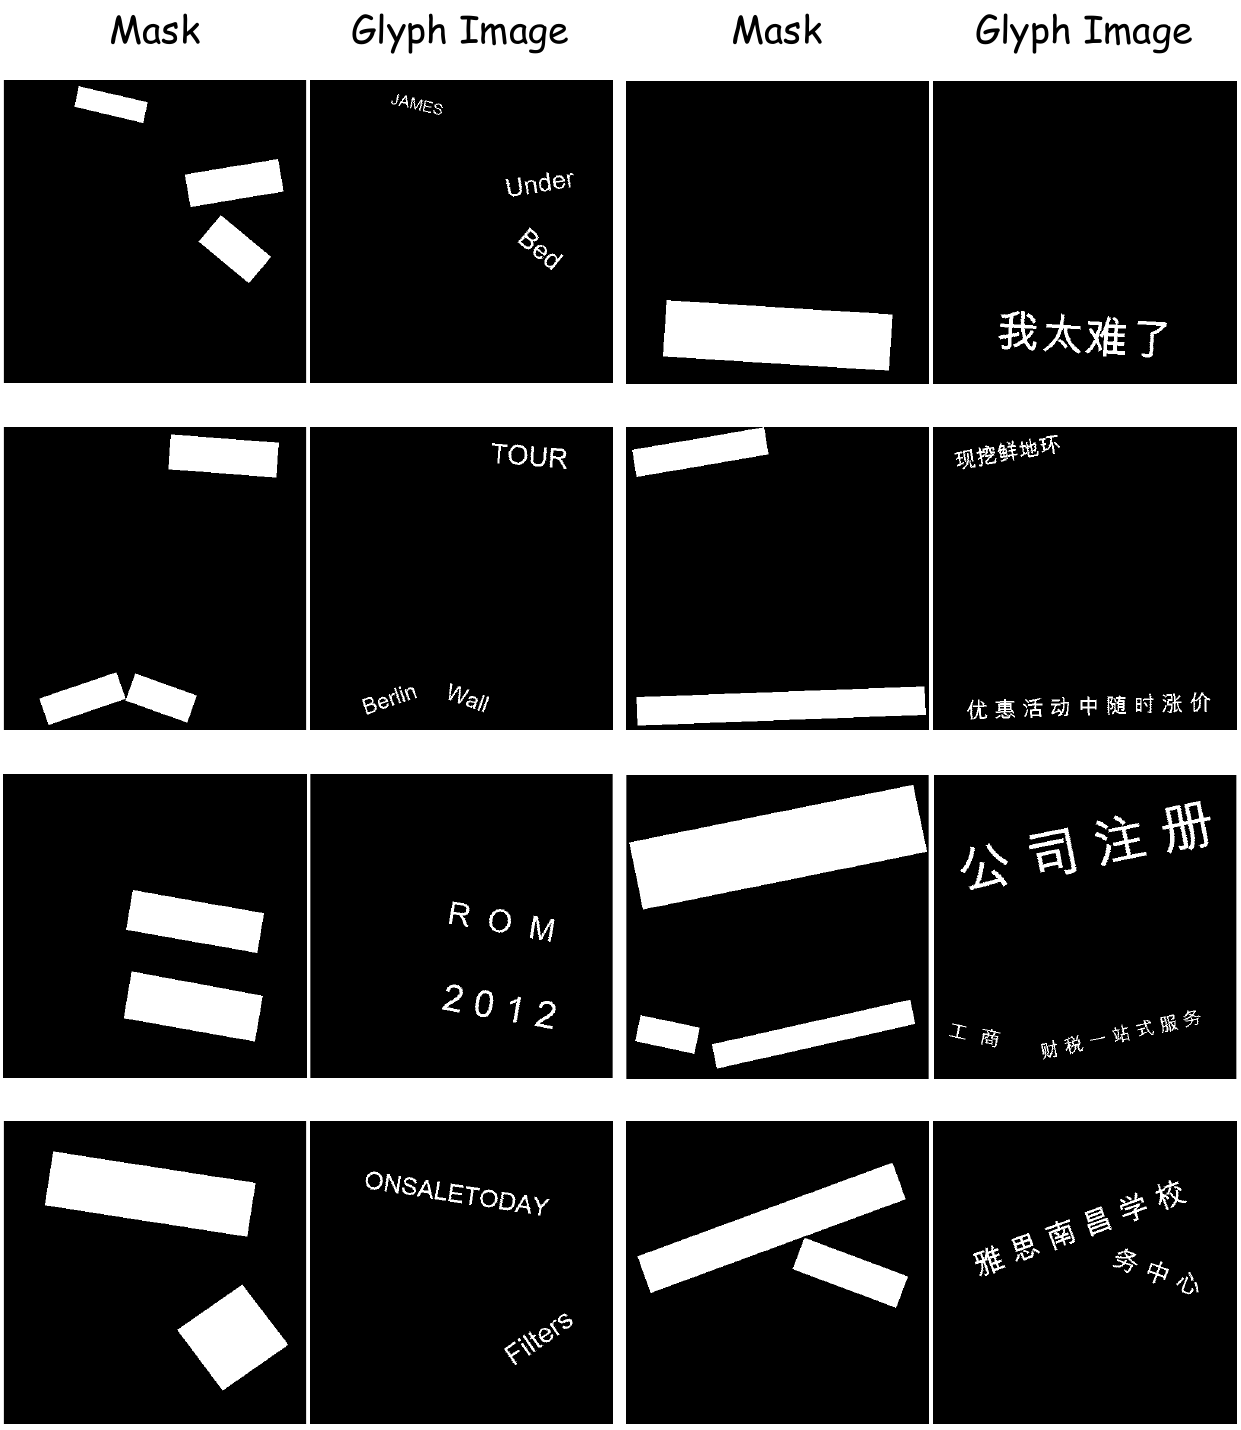}
     \caption{\textbf{Benchmark Detail.}}
     \label{fig:benchmark_detail}
\end{figure*}

\begin{figure*}
    \centering
    \includegraphics[width=1.0\linewidth]{images/user_studyv4.png}
    \vspace{-10pt}
    \caption{\textbf{User study print screen.}}
    \vspace{-10pt}
    \label{fig:user_study}
\end{figure*}
